# Supplementary material for: SonarSnoop: Active Acoustic Side-Channel Attacks
Source: arXiv:1808.10250 source file (2018-08-30)
Supplement: Supplementary file 1 [file appendix.tex]

\section*{Appendix}
\section{Machine Learning Algorithms}\label{sec:ap_machine_learning_algorithms}

\begin{table}[ht]
    %\small
    %\scriptsize
    \footnotesize
    \centering
    \begin{tabular}{|l|l|}
        \hline
        \multicolumn{1}{|c|}{\textbf{Microphones}} & \multicolumn{1}{c|}{\textbf{Algorithm}}                                                                     \\ \hline
        Both                             & \begin{tabular}[c]{@{}l@{}}Medium Gaussian SVM\\ Kernel function: Gaussian\\ Kernel scale: 2.2\end{tabular} \\ \hline
        Bottom                                 & \begin{tabular}[c]{@{}l@{}}Quadratic SVM\\ Kernel function: Quadratic\\ Kernel scale: Auto\end{tabular}           \\ \hline
        Top                                 & \begin{tabular}[c]{@{}l@{}}Quadratic SVM\\ Kernel function: Quadratic\\ Kernel scale: Auto\end{tabular} \\ \hline
    \end{tabular}
    \caption{Machine learning algorithms that have the best performance for decision method D1 when using both microphones, bottom microphone only, and top microphone only.}
    \label{tab:ap_features_algorithms}
\end{table}

\begin{table}[ht]
    %\small
    %\scriptsize
    \footnotesize
    \centering
    \begin{tabular}{|l|l|}
        \hline
        \textbf{Group of Strokes} & \multicolumn{1}{c|}{\textbf{Algorithm}}                                                                                                        \\ \hline
        2, 5, 6                             & \begin{tabular}[c]{@{}l@{}}Medium Gaussian SVM\\ Kernel function: Gaussian\\ Kernel scale: 2.2\end{tabular}                                    \\ \hline
        3, 5, 14                            & \begin{tabular}[c]{@{}l@{}}Wighted KNN\\ Number of neighbours: 10\\ Distance metric: Euclidean\\ Distance weight: Squared inv.\end{tabular} \\ \hline
        1, 11                             & \begin{tabular}[c]{@{}l@{}}Coarse Gaussian SVM\\ Kernel function: Gaussian\\ Kernel scale: 8.9\end{tabular}                                    \\ \hline
        5, 12                               & \begin{tabular}[c]{@{}l@{}}Fine KNN\\ Number of neighbours: 1\\ Distance metric: Euclidean\\ Distance weight: Equal\end{tabular}               \\ \hline
        4, 13                                & \begin{tabular}[c]{@{}l@{}}Ensemble - Bagged Trees\\ Maximum number of splits: 11\\ Number of learners: 30\end{tabular}                        \\ \hline
    \end{tabular}
    \caption{Machine learning algorithms with the best performance to classify the group of strokes in decision method D3 when using both microphones.}
    \label{tab:ap_features_algorithms_groups_both}
\end{table}

\begin{table}[ht]
    %\small
    %\scriptsize
    \footnotesize
    \centering
    \begin{tabular}{|l|l|}
        \hline
        \textbf{Group of Strokes} &  \multicolumn{1}{c|}{\textbf{Algorithm}}                                                                                                           \\ \hline
        2, 5, 6, 9                & \begin{tabular}[c]{@{}l@{}}Medium Gaussian SVM\\ Kernel function: Gaussian\\ Kernel scale: 2.2\end{tabular}                      \\ \hline
        3, 5, 7, 14             & \begin{tabular}[c]{@{}l@{}}Medium Gaussian SVM\\ Kernel function: Gaussian\\ Kernel scale: 2.2\end{tabular}                      \\ \hline
        4, 8                & \begin{tabular}[c]{@{}l@{}}Cosine KNN\\ Number of neighbours: 10\\ Distance metric: Cosine\\ Distance weight: Equal\end{tabular} \\ \hline
        1, 11                 & \begin{tabular}[c]{@{}l@{}}Coarse Gaussian SVM\\ Kernel function: Gaussian\\ Kernel scale: 8.9\end{tabular}                      \\ \hline
        5, 12                 & \begin{tabular}[c]{@{}l@{}}Medium Gaussian SVM\\ Kernel function: Gaussian\\ Kernel scale: 2.2\end{tabular}                      \\ \hline
        4, 13              & \begin{tabular}[c]{@{}l@{}}Fine KNN\\ Number of neighbours: 1\\ Distance metric: Euclidean\\ Distance weight: Equal\end{tabular} \\ \hline
    \end{tabular}
    \caption{Machine learning algorithms that have the best performance to classify the group of strokes in decision method D3 when using bottom microphone only.}
    \label{tab:ap_features_algorithms_groups_bottom}
\end{table}

\begin{table}[ht]
    %\small
    %\scriptsize
    \footnotesize
    \centering
    \begin{tabular}{|l|l|}
        \hline
        \textbf{Group of Strokes} & \multicolumn{1}{c|}{\textbf{Algorithm}}                                                                                                                  \\ \hline
        1, 3, 5, 14               & \begin{tabular}[c]{@{}l@{}}Medium KNN\\ Number of neighbours: 10\\ Distance metric: Euclidean\\ Distance weight: Equal\end{tabular} \\ \hline
        2, 4, 5, 6              & \begin{tabular}[c]{@{}l@{}}Ensemble - Bagged Trees\\ Maximum number of splits: 11\\ Number of learners: 30\end{tabular}             \\ \hline
        1, 11               & \begin{tabular}[c]{@{}l@{}}Fine Gaussian SVM\\ Kernel function: Gaussian\\ Kernel scale: 0.56\end{tabular}                          \\ \hline
        5, 12               & \begin{tabular}[c]{@{}l@{}}Cosine KNN\\ Number of neighbours: 10\\ Distance metric: Cosine\\ Distance weight: Equal\end{tabular}    \\ \hline
        4, 13               & \begin{tabular}[c]{@{}l@{}}Quadratic SVM\\ Kernel function: Quadratic\\ Kernel scale: Auto\end{tabular}                             \\ \hline
        1, 7              & \begin{tabular}[c]{@{}l@{}}Ensemble - Bagged Trees\\ Maximum number of splits: 11\\ Number of learners: 30\end{tabular}             \\ \hline
        8, 9               & \begin{tabular}[c]{@{}l@{}}Coarse Gaussian SVM\\ Kernel function: Gaussian\\ Kernel scale: 8.9\end{tabular}                         \\ \hline
    \end{tabular}
    \caption{Machine learning algorithms that have the best performance to classify the group of strokes in decision method D3 when using top microphone only.}
    \label{tab:ap_features_algorithms_groups_top}
\end{table}
